# Supplementary material for: Inversion of the exciton built-in dipole moment in In(Ga)As quantum dots via nonlinear piezoelectric effect
Source: arXiv:1702.08314 ancillary file (2017-08-07)
Supplement: Supplementary file 1 [file Supplemental_Material.pdf]

## Supplemental Material for:

# Inversion of the exciton built-in dipole moment in In(Ga)As quantum dots via nonlinear piezoelectric effect

Johannes Aberl,[1,*] Petr Klenovský,[2,3,†] Johannes S. Wildmann,[1] Javier Martín-Sánchez,[1] Thomas Fromherz,[1] Eugenio Zallo,[4,5] Josef Humlíček,[2,3] Armando Rastelli,[1] and Rinaldo Trotta[1,‡]

[1] *Institute of Semiconductor and Solid State Physics, Johannes Kepler University Linz, Altenbergerstraße 69, A-4040 Linz, Austria*
[2] *Department of Condensed Matter Physics, Masaryk University, Kotlářská, CZ-61137 Brno, Czech Republic*
[3] *Central European Institute of Technology, Masaryk University, Kamenice 753/5, CZ-62500 Brno, Czech Republic*
[4] *Institute for Integrative Nanosciences, IFW Dresden, Helmholtzstraße 20, D-01069 Dresden, Germany*
[5] *Paul-Drude-Institut für Festkörperelektronik, Hausvogteilplatz 5-7, 10117 Berlin, Germany*

(Dated: June 1, 2017)

**Contents**

**I. Complete measurement data** 2

**II. Determination of the angle between major stress axis and [110] direction** 3

**III. Determination of magnitude and anisotropy of the applied stress** 4

**IV. Calculation of the effect of the interface charge on the potential in doped semiconductors** 4

**V. Discussion of the used diode model** 7

**VI. Effect of various piezoelectric coefficients** 9

**VII. Effect of self-consistency calculations** 10

**References** 10

---

* johannes.aberl@jku.at
† klenovsky@physics.muni.cz
‡ rinaldo.trotta@jku.at

# I. COMPLETE MEASUREMENT DATA

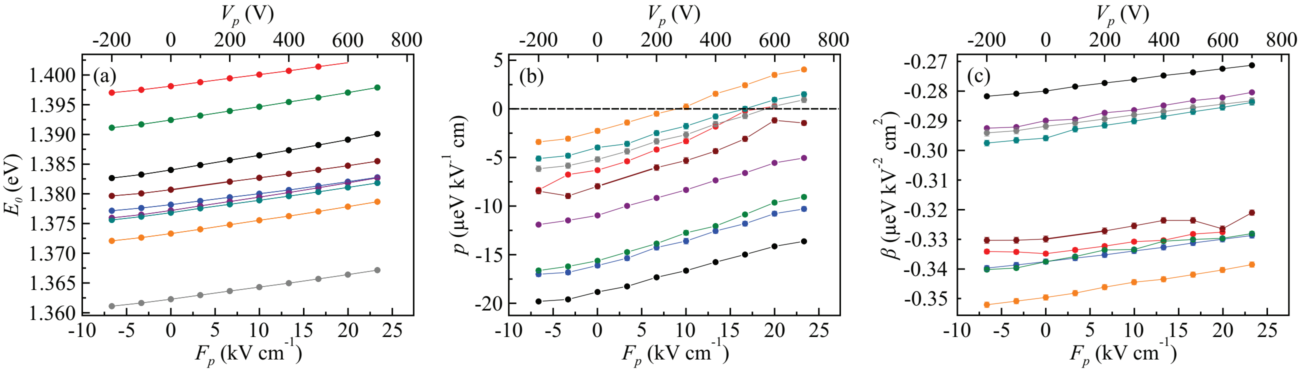


FIG. 1: Zero-field transition energy $E_0$ (a), built-in dipole moment $p$ (b) and polarizability $\beta$ (c) as a function of the voltage applied to the PMN-PT piezoelectric actuator $V_p$ (electric field across the PMN-PT $F_p$, respectively) for all measured $X$s.

The data provided in the main letter, highlighting the inversion of the exciton built-in dipole moment, represent just a meaningful excerpt of the totally measured. We extracted zero-field transition energy $E_0$, built-in dipole moment $p$ and polarizability $\beta$ of excitons $X$, biexcitons $XX$, positive- and negative trions $X^+$, $X^-$ for different $V_p$ by fitting the corresponding micro-photoluminescence spectra.
In Fig. 1(a)–Fig. 1(c) we provide the full set of obtained parameters, covering the full tuning range of $V_p$, for all measured $X$s. The observed linear shift of $E_0$ with applied stress (see Fig. 1(a)) is consistent with Refs. [1, 2]. As emphasized in the letter, all $X$s show negative $p$ at zero-stress applied (i.e. $F_p = 0$). Considering the orientation of the QDs in our structure ("upside-down" because of the device processing), this indicates that the mean position of the electron is closer to the QD's base and the hole tends to be located closer to the apex. As apparent from Fig. 1(b), electron and hole approach each other under compression (i.e. $F_P > 0$). The obtained linear shift of $p$ with applied stress was observed for all measured $X$s and for 4 out of 9 investigated QDs we achieved an inversion of the electron-hole alignment (i.e. a sign change of $p$). Similar to $E_0$ and $p$, the polarizability $\beta$ shows a linear trend as well (see Fig. 1(c)), albeit the relative variation is rather small.

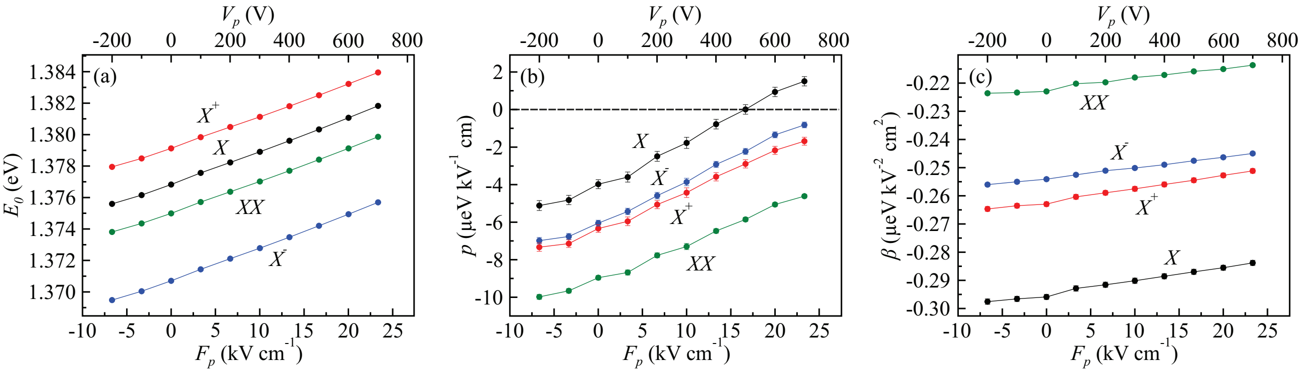


FIG. 2: Obtained results for zero-field transition energy $E_0$ (a), built-in dipole moment $p$ (b) and polarizability $\beta$ (c) as a function of the voltage applied to the PMN-PT piezoelectric actuator $V_p$ (electric field across the PMN-PT $F_p$, respectively) for exciton $X$ (black), biexciton $XX$ (green), positive $X^+$ (red) and negative trion $X^-$ (blue) of one QD.

As already mentioned, similar data analysis was performed for all the other few-particle states. $E_0$, $p$ and $\beta$ obtained for $X$, $XX$, $X^+$ and $X^-$ of one QD are reported in Fig. 2(a)–Fig. 2(c). The zero-stress values $\langle f(F_p = 0)\rangle$, slopes $\langle df/dF_p\rangle$ and tuning ranges $\langle \Delta f\rangle$ ($f$ representing $E_0$, $p$ or $\beta$) averaged over all measured $X$, $XX$, $X^+$ and $X^-$ respectively, are given in Tab. I. On average, excitons show significantly lower magnitude of $p$ in comparison to $XX$, $X^+$ and $X^-$. In contrary, average slope and tuning range are both highest for $X$. While this effect can be rationalized

taking into account the number of carriers composing the excitonic complexes and the strain-induced changes of the Coulomb interaction energies, a detailed discussion is beyond the scope of the present work.

| | $f(F_p)$ | zero-stress $\langle f(F_p = 0)\rangle$ | slope $\langle df/dF_p\rangle$ | tuning range $\langle \Delta f\rangle$ |
|---|---|---|---|---|
| $X$ | $E_0$ | (1.38 ± 0.02) eV | $(0.21 \pm 0.02)$ meV kV$^{-1}$ cm | $(6.3 \pm 0.8)$ meV |
| | $p_z$ | (-10 ± 6) $\mu$eV kV$^{-1}$ cm | $(0.26 \pm 0.04)$ $\mu$eV kV$^{-2}$ cm$^2$ | $(7.2 \pm 0.7)$ $\mu$eV kV$^{-1}$ cm |
| | $\beta$ | (-0.32 ± 0.03) $\mu$eV kV$^{-2}$ cm$^2$ | $(0.38 \pm 0.07)$ neV kV$^{-3}$ cm$^3$ | $(11.1 \pm 2.3)$ neV kV$^{-2}$ cm$^2$ |
| $XX$ | $E_0$ | (1.38 ± 0.01) eV | $(0.21 \pm 0.01)$ meV kV$^{-1}$ cm | $(6.1 \pm 0.1)$ meV |
| | $p$ | (-13 ± 6) $\mu$eV kV$^{-1}$ cm | $(0.21 \pm 0.04)$ $\mu$eV kV$^{-2}$ cm$^2$ | $(5.8 \pm 0.8)$ $\mu$eV kV$^{-1}$ cm |
| | $\beta$ | (-0.25 ± 0.02) $\mu$eV kV$^{-2}$ cm$^2$ | $(0.33 \pm 0.08)$ neV kV$^{-3}$ cm$^3$ | $(9.6 \pm 2.9)$ neV kV$^{-2}$ cm$^2$ |
| $X^+$ | $E_0$ | (1.38 ± 0.01) eV | $(0.20 \pm 0.03)$ meV kV$^{-1}$ cm | $(6.1 \pm 0.7)$ meV |
| | $p$ | (-15 ± 7) $\mu$eV kV$^{-1}$ cm | $(0.21 \pm 0.05)$ $\mu$eV kV$^{-2}$ cm$^2$ | $(5.9 \pm 1.1)$ $\mu$eV kV$^{-1}$ cm |
| | $\beta$ | (-0.27 ± 0.03) $\mu$eV kV$^{-2}$ cm$^2$ | $(0.44 \pm 0.02)$ neV kV$^{-3}$ cm$^3$ | $(12.8 \pm 4.7)$ neV kV$^{-2}$ cm$^2$ |
| $X^-$ | $E_0$ | (1.38 ± 0.01) eV | $(0.22 \pm 0.02)$ meV kV$^{-1}$ cm | $(6.5 \pm 0.8)$ meV |
| | $p$ | (-12 ± 7) $\mu$eV kV$^{-1}$ cm | $(0.25 \pm 0.05)$ $\mu$eV kV$^{-2}$ cm$^2$ | $(6.7 \pm 1.3)$ $\mu$eV kV$^{-1}$ cm |
| | $\beta$ | (-0.27 ± 0.02) $\mu$eV kV$^{-2}$ cm$^2$ | $(0.23 \pm 0.25)$ neV kV$^{-3}$ cm$^3$ | $(6.3 \pm 7.7)$ neV kV$^{-2}$ cm$^2$ |

TABLE I: Averaged values for the parameters $E_0$, $p$ and $\beta$ measured at $F_p = 0$, the average tuning ranges as well as the corresponding averaged slopes for the all few-particle states $X$, $XX$, $X^+$ and $X^-$.

## II. DETERMINATION OF THE ANGLE BETWEEN MAJOR STRESS AXIS AND [110] DIRECTION

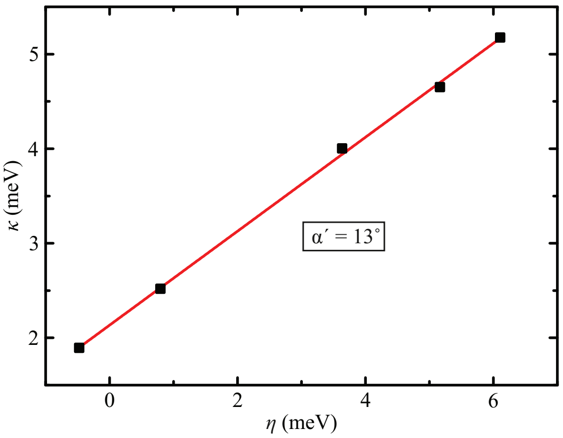


FIG. 3: Behavior of $\kappa$ as a function of $\eta$ for one of the investigated QDs. The value of the angle $\alpha'$ (with respect to the [110] direction) as estimated with Eq. (1) is also reported.

The behavior of the FSS ($s$) and the polarization angle of the $X$ emission ($\gamma$) vs the voltage applied to the PMN-PT $V_p$ can be explained by a theoretical model developed for the exciton Hamiltonian $H$ which takes into account the effect of in-plane stresses of variable magnitudes, directions and anisotropies (see Ref. 3). This theoretical model can be used to determine the direction of the applied stress and in particular the angle $\alpha'$ between the major stress axis ($S_1$) and the [110] direction. We refer the reader to Refs. [3], [4] for details on the model and we provide here only the final result for the angle $\alpha'$, which reads

$$\tan(2\alpha') \approx \frac{\kappa - \kappa_0}{\eta - \eta_0}. \tag{1}$$

where $\eta = s\sin(2\gamma)/2$, $\kappa = s\cos(2\gamma)/2$ and $\eta_0$ and $\kappa_0$ are the same values for zero applied stress. Figure 3 shows the behavior of $\kappa$ as a function of $\eta$ when the voltage $V_p$ is swept. All points lie on straight line (the values of these parameters match previous theoretical calculations performed for similar QDs, see Refs. [4], [5]). By using Eq. (1) we find $\alpha' = 13.2°$ ($\alpha = 58.2°$) with respect to the [110] ([100]) direction. We have repeated this procedure for different QDs and the average value we find is $\alpha = 58.3 \pm 4.2°$. Considering the error, we have used $\alpha = 55°$ ($\alpha' = 10°$) in the calculations below.

## III. DETERMINATION OF MAGNITUDE AND ANISOTROPY OF THE APPLIED STRESS

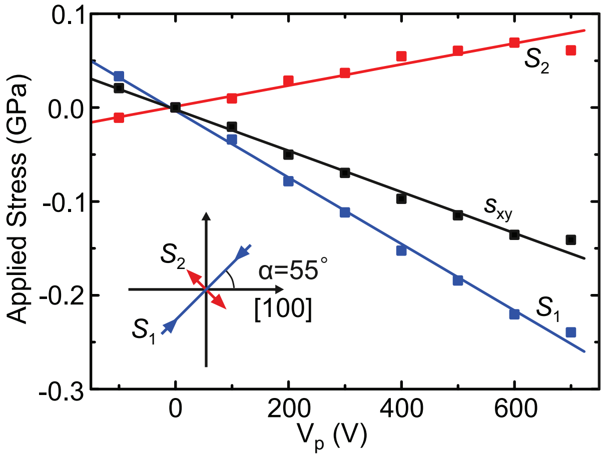


FIG. 4: Major ($S_1$), minor ($S_2$) and shear stress ($s_{xy}$) as a function of the voltage applied to the piezoelectric actuator ($V_p$). The full data points show the values estimated from the experimental data while the solid lines show the result of the simulations as obtained with $S_1/S_2 = -3.16$ and $\alpha = 55°$. The calculated stress configuration for positive $V_p$ is schematically depicted in the inset.

As mentioned in the main text, the complete determination of the in-plane stress delivered by the PMN-PT actuator requires knowledge of three independent parameters: $S_1$, $S_2$ and $\alpha$. In the previous section we have determined $\alpha$ using the magnitude of the FSS and the polarization direction of the exciton emission. With this value now at hand, we can calculate $S_1$ and $S_2$ (and therefore magnitude and anisotropy of the applied stress) via the strain-induced shift of the $X$ transition and of the $I$-$V$ trace onset. The results of these calculations are shown in Fig. 4 (see the main text for the formulas we have used), where the values of $S_1$ and $S_2$ are reported for each $V_p$ (full squares). For completeness, we reported also the value of the shear stress ($s_{xy}$), which we remind is related to $S_1$ and $S_2$ via $s_{xy} = \frac{S_1 - S_2}{2}\sin(2\alpha)$. Assuming a linear dependence between $S_1$ and $V_p$ we can simulate the experimental data over the whole tuning range with $S_1/S_2 = -3.16$ (see the solid lines). Therefore, the stress delivered by our piezoelectric actuator results to be strongly anisotropic with $S_1$ ($S_2$) being compressive (tensile) for positive (negative) $V_p$. This in-plane strain configuration, which we use to perform the $\mathbf{k}\cdot\mathbf{p}$ calculations shown in the main text, is schematically shown in the inset of Fig. 4.
It is worth emphasizing that the values reported in Fig. 4 correspond to the applied stress and do not take into account the presence of the pre-stress at $V_p = 0$. As discussed in the main text, the latter is estimated by reproducing the value of the dipole moment at $V_p = 0$ during the $\mathbf{k}\cdot\mathbf{p}$ calculations. As the dipole moment for the given QD shape is sensitive only to the shear component of the stress, we can estimate $s_{xy} = 0.2\,\text{GPa}$ only. In turn, this value can be effectively reproduced by assuming the following strain configuration $S_1^{pre} = -S_2^{pre} = 0.2\,\text{GPa}$ and $\alpha^{pre} = 0$, which can be added to the applied stress to obtain the absolute stress configuration. It is important to point out that the assumption on the pre-stress has no role in the strain-induced shift of the dipole moment, which is fully determined by the applied stress we have extracted from the experimental data (see Fig. 4).

## IV. CALCULATION OF THE EFFECT OF THE INTERFACE CHARGE ON THE POTENTIAL IN DOPED SEMICONDUCTORS

We consider here the effect produced by piezoelectricity on the Schottky barrier at the interface between an n-doped semiconductor and a metal contact. We begin the discussion by recalling the properties of a metal-semiconductor interface. The one-dimensional Poisson equation (in SI units) reads

$$\frac{\mathrm{d}^2\varphi(z)}{\mathrm{d}z^2} = -\frac{\rho_e(z)}{\varepsilon\varepsilon_0}, \tag{2}$$

where $\varphi(z)$ is the potential and $\rho_e(z)$ is the corresponding volume charge; $\varepsilon$ and $\varepsilon_0$ are the relative and vacuum permittivities, respectively. In equilibrium, the concentration $c(z)$ of free carriers is related to the density of states

$D(E, z)$, assuming a parabolic dispersion of the electron energies E, by

$$D(E, z) = \frac{\sqrt{2}}{\pi^2} \frac{(m_0 m^*)^{3/2}}{\hbar^3} \sqrt{E - E_c(z)}, \tag{3}$$

for $E \geq E_c$. Here $m^*$ is the dimensionless effective mass in the band, $m_0$ the free electron mass, and $E_c(z)$ the conduction band-edge energy related to the electrostatic potential $\varphi(z)$ by

$$E_c(z) = E_{cB} - e\varphi(z), \tag{4}$$

where $E_{cB}$ is the conduction band edge in the bulk of the semiconductor and $e$ is the absolute value of the electron charge. Taking into account the Fermi-Dirac statistics and Eq. (4) we arrive at the formula for the concentration of the electrons

$$c(z) = \frac{\sqrt{2kT}}{\pi^2} \frac{(m_0 m^*)^{3/2}}{\hbar^3} \cdot \int_0^\infty \frac{\sqrt{E/kT}}{\exp \frac{E - (e\varphi(z) + E_F - E_{cB})}{kT} + 1} \mathrm{d}E. \tag{5}$$

where $E_F$ is the Fermi energy, $k$ the Boltzmann constant and $T$ the temperature. On the right hand side we have the Fermi-Dirac integral $\mathcal{F}_{1/2}((e\varphi(z) + E_F - E_{cB})/kT)$. It is convenient to use the following dimensionless variables

$$u(z) = \frac{e\varphi(z)}{kT}, \ \xi = (E_F - E_{cB})/kT, \ t = E/kT. \tag{6}$$

Inserting them into Eq. (5) we obtain

$$c(z) = \frac{\sqrt{2}}{\pi^2} \frac{(kTm_0 m^*)^{3/2}}{\hbar^3} \cdot \int_0^\infty \frac{\sqrt{t}}{\exp[t - (u(z) + \xi)] + 1} \mathrm{d}t = N_d \cdot \mathcal{F}_{1/2}(u(z) + \xi), \tag{7}$$

where $N_d = \sqrt{2}(kTm_0 m^*)^{3/2}/(\pi^2 \hbar^3)$ is the effective density of states. Assuming an n-doped semiconductor with fully ionized donors with density $n_d$, the volume charge density produced due to the presence of the interface is given by

$$\rho_e(z) = e(n_d - c(z)), \tag{8}$$

where $c(z)$ is given by Eq. (7) and $n_d = c(-\infty)$ is the electron concentration in the bulk (far away from the interface). In bulk the impact of the surface potential is negligible so $\varphi(-\infty) = 0$ and thus $u(-\infty) = 0$, consequently

$$n_d = N_d \cdot \mathcal{F}_{1/2}(\xi). \tag{9}$$

We insert Eq. (8) into Eq. (2) to obtain the Poisson equation for $u$:

$$\frac{\mathrm{d}^2 u(z)}{\mathrm{d}z^2} = \frac{e}{kT} \frac{\mathrm{d}^2 \varphi(z)}{\mathrm{d}z^2} = -\frac{e}{\varepsilon\varepsilon_0 kT} \rho_e(z). \tag{10}$$

Combining that with Eqs. (7) and (8) we arrive at

$$\begin{aligned} \frac{\mathrm{d}^2 u(z)}{\mathrm{d}z^2} &= -\frac{e}{\varepsilon\varepsilon_0 kT} [ec(-\infty) - ec(z)] = -\frac{e^2 N_d \mathcal{F}_{1/2}(\xi)}{\varepsilon\varepsilon_0 kT} \cdot \left[1 - \frac{\mathcal{F}_{1/2}(u(z) + \xi)}{\mathcal{F}_{1/2}(\xi)}\right] \\ &= -\frac{1}{L_d^2} \left[1 - \frac{\mathcal{F}_{1/2}(u(z) + \xi)}{\mathcal{F}_{1/2}(\xi)}\right], \end{aligned} \tag{11}$$

where $L_d$ is the Debye screening length

$$L_d = \sqrt{\frac{\varepsilon\varepsilon_0 kT}{e^2 n_d}} \tag{12}$$

for the dopant concentration $n_d = c(-\infty) = N_d \mathcal{F}_{1/2}(\xi)$. We now have to solve Eq. (11) in order to extract the slope $\mathrm{d}u/\mathrm{d}z$. Taking into account the property of Fermi-Dirac integrals

$$\frac{\mathrm{d}\mathcal{F}_n(\eta)}{\mathrm{d}\eta} = n\mathcal{F}_{n-1}(\eta), \tag{13}$$

it is easy to show that the solution of Eq. (11) satisfies the following relation:

$$\left(\frac{\mathrm{d}u(z)}{\mathrm{d}z}\right)^2 = \frac{2}{L_d^2}\left[-u(z) + \frac{2}{3}\frac{\mathcal{F}_{3/2}(u(z)+\xi) - \mathcal{F}_{3/2}(\xi)}{\mathcal{F}_{1/2}(\xi)}\right]. \tag{14}$$

This can be rewritten in a compact form

$$\frac{\mathrm{d}u(z)}{\mathrm{d}z} = \frac{\sqrt{2}}{L_d}\mathcal{F}(u(z),\xi), \tag{15}$$

where

$$\mathcal{F}(u(z),\xi) = \sqrt{-u(z) + \frac{2}{3}\frac{\mathcal{F}_{3/2}(u(z)+\xi) - \mathcal{F}_{3/2}(\xi)}{\mathcal{F}_{1/2}(\xi)}}. \tag{16}$$

Combining Eqs. (2) and (11) having in mind the definition of $u(z)$ in the first of Eqs. (6) we can see that $\rho_e$ as a

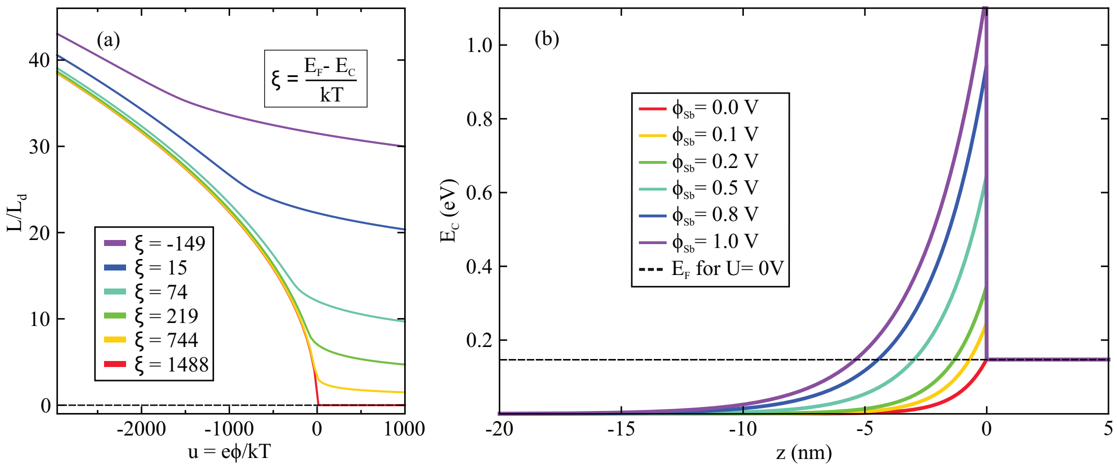


FIG. 5: (a) Effective screening length L normalized to Debye length $L_d$ for depletion ($u < 0$) and accumulation ($u > 0$) layer as a function of the potential $\phi$ at the semiconductor-metal interface. The dependencies are plotted for several values of ($E_F$-$E_c$)/kT. (b) Energy of the electrons as a function of the distance from the semiconductor-metal interface. The dependencies are plotted for several Schottky barrier heights, the Fermi level is shown by dotted line.

function of $z$ reads

$$\rho_e(z) = -\frac{\varepsilon\varepsilon_0 kT}{e}\frac{\mathrm{d}^2u(z)}{\mathrm{d}z^2} = en_d\left[1 - \frac{\mathcal{F}_{1/2}(u(z)+\xi)}{\mathcal{F}_{1/2}(\xi)}\right]. \tag{17}$$

The potential $u(0)$ at the interface can be connected to the sheet charge density $\sigma$, which is obtained by integrative the volume charge density over the z direction integrating Eq. (17) from $-\infty$ to 0 and taking into account Eq. (15), we obtain

$$\sigma = -\sqrt{2n_d\varepsilon\varepsilon_0 kT}\sqrt{-u(0) + \frac{2}{3}\frac{\mathcal{F}_{3/2}(u(0)+\xi) - \mathcal{F}_{3/2}(\xi)}{\mathcal{F}_{1/2}(\xi)}}. \tag{18}$$

A potential difference between the semiconductor and the metal originates from the difference of their work functions. In a close contact, this potential drop manifests itself as e.g. the Schottky barrier, thin insulating layer, or others, see Refs. 6, 7. The arrangement depends on the particular metal and semiconductor, the surface of the semiconductor and the quality of the contact itself. We will restrict ourselves to the case of Schottky barrier $\phi_{sb}$, usually defined as the potential difference from the Fermi level $E_F$, see Ref. 7. At the interface ($z = 0$), we have therefore: $u(0) = -\xi + \frac{e\phi_{sb}}{kT}$. We insert this to Eq. (18) and obtain

$$\sigma_s = -\sqrt{2n_d\varepsilon\varepsilon_0 kT}\sqrt{\xi - \frac{e\phi_{sb}}{kT} + \frac{2}{3}\frac{\mathcal{F}_{3/2}(\frac{e\phi_{sb}}{kT}) - \mathcal{F}_{3/2}(\xi)}{\mathcal{F}_{1/2}(\xi)}}. \tag{19}$$

Equation (19) provides us with the sought relation between $\phi_{Sb}$ and the surface charge $\sigma_s$ which is produced at the semiconductor-metal interface. Similarly, the surface charge $\sigma_t$ produced by an additional surface potential $e\theta$ is accounted for by replacing $\phi_{Sb}$ with $\phi_{Sb} + \theta$:

$$\sigma_t = -\sqrt{2n_d\varepsilon\varepsilon_0 kT}\sqrt{\xi - \frac{e(\phi_{sb}+\theta)}{kT} + \frac{2}{3}\frac{\mathcal{F}_{3/2}(\frac{e(\phi_{sb}+\theta)}{kT}) - \mathcal{F}_{3/2}(\xi)}{\mathcal{F}_{1/2}(\xi)}}. \tag{20}$$

In order to extract the surface charge density $\sigma_p$ corresponding to the strain induced piezoelectricity we need to subtract Eqs. (20) and (19), i.e.

$$\sigma_p = \sigma_t - \sigma_s. \tag{21}$$

It is further convenient to approximate the monotonic function $u(z)$. We have chosen the exponential

$$u(z) \approx u(0)\exp(\frac{z}{L}), \tag{22}$$

where $L$ is the effective screening length. Its value may be chosen to match the derivative of Eq. (22) at the surface $\frac{\mathrm{d}u}{\mathrm{d}z}\big|_{z=0}$ satisfying Eq. (15). This is achieved with

$$L = L_d \frac{1}{\sqrt{2}}\frac{u(0)}{\mathcal{F}(u(0),\xi)}. \tag{23}$$

The screening length $L$ normalized to $L_d$ is shown in Fig. 5(a) for different energy differences between $E_F$ and $E_c$ and different interface potentials. The screening length at 7.8 K in the case of $E_F - E_c = 0.147\,\mathrm{eV}$, corresponding to the donor doping in n-type GaAs of $5{\times}10^{18}\,\mathrm{cm}^{-3}$, is 1.35 nm, almost 15.5 times larger than $L_d = 2.9$Å. In Fig. 5(b) we show the conduction band edge as a function of the distance from the interface for different Schottky barriers for $E_F - E_c$ fixed to 0.187 eV. Finally, the magnitude of the field $F_{\mathrm{qd}}$ acting on QDs, produced solely due to piezoelectricity stemming from externally induced stress, can be calculated by

$$F_{\mathrm{qd}} = \left(\frac{e_{14}^{qd}}{\varepsilon_{qd}} - \frac{\frac{\mu_{qd}}{\mu_i}e_{14}^{i}}{\varepsilon_i}\right)\frac{\sigma_{xy}^{qd}}{C_{44}}, \tag{24}$$

where $\varepsilon$ is the dielectric constant and $\mu$ the shear modulus. The sub- and super-scripts $qd$ and $i$ represent the materials of the layer where the dots reside (GaAs) and that of the rest of the intrinsic region ($Al_{0.4}Ga_{0.6}As$), respectively. In derivation of Eq. (24) we have assumed that the interfaces of all layers in our structure are infinite. Furthermore, we must fulfill the boundary conditions for the potential at the edges of the p-i-n diode, resulting in a multiplication of Eq. 24 by a correction factor of $(1 - L_{qd}/L_i)$, where the lengths $L_i$ and $L_{qd}$ are defined in Fig. 6.

## V. DISCUSSION OF THE USED DIODE MODEL

The band diagram for the studied diode [n-GaAs (178 nm) / n-$Al_{0.4}Ga_{0.6}As$ (30.5 nm) / i-$Al_{0.4}Ga_{0.6}As$ (70 nm) / i-GaAs (10 nm) / i-$Al_{0.4}Ga_{0.6}As$ (70 nm) / p-$Al_{0.4}Ga_{0.6}As$ (30.5 nm) / p-GaAs (71 nm)]) is shown in Fig. 6 for different bias conditions. According to the model described in the previous section, the Au top-contact to the p-i-n diode (containing the QDs) acts as a Schottky diode which is biased in reverse direction if the p-i-n diode is biased in forward direction (see Fig. 6(a)) and vice versa (see Fig. 6(b)). At the bias points shown in Fig. 1(c) of the main paper, at which the differential resistance of the two-diode system is strongly reduced, the current has to tunnel through the Schottky contact as it is biased in reverse direction. The same current has to pass the p-i-n diode as diffusion current determined by the minority carrier concentration at the borders of the space charge region. Since these concentrations are in turn determined by the energy differences between the quasi-Fermi-levels ($e\phi_p$, $e\phi_n$) and the respective minority carrier bands ($E_c$ on p-side, $E_v$ on n-side), for equal currents through the device these positions must be equal. As a consequence, only a strain-induced change of the bandgap of the p- and n-$Al_{0.4}Ga_{0.6}As$ regions $E_g^A$ in our device would modify the voltage drop over the p-i-n diode for a constant current, but not the strain-induced piezoelectric polarization. However, in Fig. 1(c) of the main paper it is shown, that, in order to maintain a constant current through the device for different applied stress (i.e. different $F_p$ applied to the PMN-PT), we need to change the voltage $V_d$ applied across Schottky contact and p-i-n junction approximately 15 times more than $E_g^A/e$ changes (as monitored by the $X$ emission). Thus, we conclude that the voltage shifts required to maintain a constant current through our device mainly drop over the Schottky contact whereby the barrier height $\phi_{Sb}$ is assumed to vary with applied stress

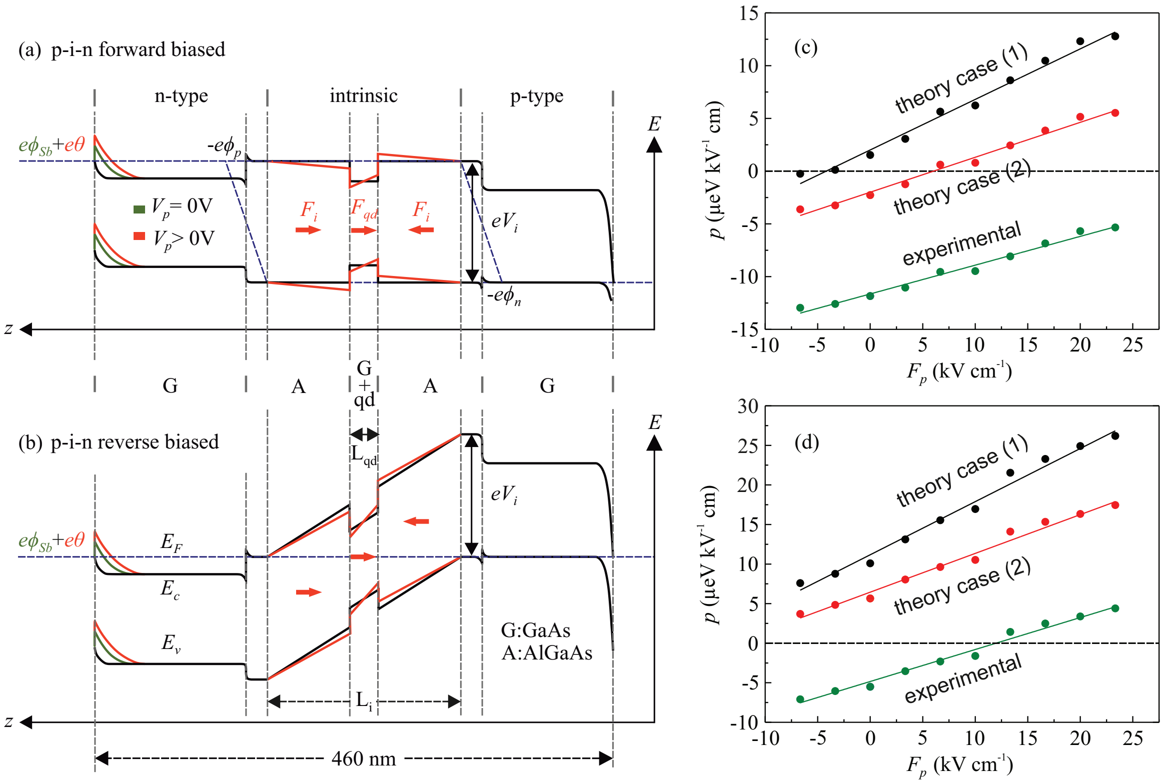


FIG. 6: Schematic band profiles of the studied device are shown for the p-i-n diode in forward bias (a) and in reverse bias (b). The used variables are defined in the text. The $X$ dipole moment $p$ for two different QDs is shown in (c) and (d) as a function of $F_p$. Hereby the total electric field $F_d$ at the QD position was calculated using the two limiting cases (1. black, 2. red) of our diode model (assuming $\phi_{Sb} = 0.1\,\mathrm{V}$ and neglecting the present pre-stress) as well as via an effective (strain-dependent) built-in voltage estimated from the current onset (green) as described in the paper.

[8]. As a consequence, for an external voltage polarity driving the Schottky diode into reverse direction, one has to subtract the strain-induced changes of the voltage drop over the Schottky contact from the externally applied bias voltage $V_d$ in order to estimate the contribution of the bias voltage on the total electric field $F_d$ at the position of the QDs. For the bias condition during the PL measurements, i.e. for voltages driving the p-i-n diode in reverse direction the situation is much less defined. Only the small saturation current of the p-i-n diode traverses the Schottky contact in this situation and the required voltage drop across the Schottky diode is unknown. Two limiting situations can be envisaged:

1. If the $I$-$V$ characteristics of the Schottky diode has a kink-like shape with approximately infinite (zero) differential resistance for voltages below (above) the Schottky barrier, the strain-dependent Schottky barrier must be subtracted from the externally applied bias $V_d$ in order to derive the voltage drop across the p-i-n junction. It is therefore reasonable to estimate $F_d$ via

$$F_d = \frac{V_d + (\phi_{sb} + \theta) + V_i}{d_d} + F_{qd} \qquad (25)$$

   where $\phi_{Sb} + \theta$ is the strain-dependent Schottky barrier, $V_i = E_g^A/e \approx 2\,\mathrm{V}$ corresponds to the $Al_{0.4}Ga_{0.6}As$ bandgap at low temperature [9], $F_{qd}$ is the additional (piezoelectric) field acting on the QDs (see previous section) and $d_d = 150\,\mathrm{nm}$ the thickness of the intrinsic region of the p-i-n diode.

2. If the saturation current of the p-i-n diode is much smaller than the saturation current of the Schottky diode, the voltage drop across the Schottky diode is small and in good approximation the externally applied voltage drops almost entirely across the p-i-n diode. In this case it would be convenient to calculate $F_d$ via

$$F_d = \frac{V_d + V_i}{d_d} + F_{qd}. \quad (26)$$

Although $\phi_{Sb} + \theta$ can be neglected here, the field $F_{qd}$ has to be included as it is independent of the voltage drop across Schottky contact.

As indicated in the paper, the determination of $p$ is tightly connected to the calculation of $F_d$. In this context it is worth mentioning, that, while the discussed diode model allows us to calculate the applied stress for each $F_p$ looking at the *relative* shift of the $I$-$V$ trace, a pre-stress is already present at $F_p = 0$ (i.e. no external stress applied). As described, this is a common feature that we observe in our devices [10] and can be readily noticed from the position of the current onset at $V_d \approx -1.74\,\mathrm{V}$ in the $I$-$V$ trace measured for $F_p = 0\,\mathrm{V}$. However, no quantitative information can be extracted from this value as it is influenced by many parameters, most notably the quality of the contact. Consequently the pre-stress cannot be reasonably included in the described model. Therefore the evaluation of the Stark shift was performed using the simple assumption of an effective (strain-dependent) built-in voltage $V_{bi}$ estimated from the current onset as described in the paper. In Fig. 6(c) and Fig. 6(d) we show the $X$ dipole moment $p$ as a function of $F_p$ for two different QDs. Hereby the data evaluation was additionally performed using Eq. 25 and Eq. 26 for the calculation of $F_d$. As apparent, in any case, a reversal of $p$ can be obtained as a function $F_p$ for particular QDs. Moreover, we emphasize that the change of the dipole moment is remarkable irrespective of the formula used to calculate the electric field $F_d$.

## VI. EFFECT OF VARIOUS PIEZOELECTRIC COEFFICIENTS

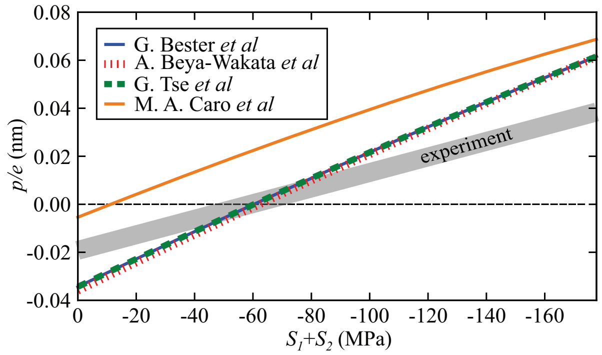


FIG. 7: Carrier separation $p/e$ in the studied QD as a function of applied stress calculated using different values for the piezoelectric coefficients $e_{14}$, $B_{114}$, $B_{124}$ and $B_{156}$ reported by G. Bester *et al* [11] (blue), A. Beya-Wakata *et al* [12] (red), G. Tse *et al* [13] (green) and M. A. Caro *et al* [14] (orange) for InAs and GaAs, respectively. All calculations where performed for the estimated stress-configuration corresponding to $\alpha = 55°$.

As mentioned in the paper, there are several theoretical works available that compute the first- and second order piezoelectric coefficients (PECs) $e_{14}$, $B_{114}$, $B_{124}$ and $B_{156}$ for various zinc-blende materials based on the framework of density functional (perturbation) theory (DFT). To account for the large discrepancies in the reported values we tested our $\mathbf{k} \cdot \mathbf{p}$ calculations for PECs provided by Refs. 11–14. The corresponding explicit values are summarized in Tab. II.

As apparent from Fig. 7, the results using PECs from Ref. 11 (used for the calculations presented in the paper) and those from Ref. 12 are quite similar, whereby the values taken from Ref. 11 still lead to a slightly better agreement with the experiment. This is no surprise as both basically follow the same methodology and the obtained PECs only differ significantly in the $B_{156}$ coefficient which is solely related to the shear part. Although the coefficients obtained in Ref. 13 widely disagree (in particular $e_{14}$ and $B_{124}$) with those reported in Refs. 11 and 14, the overall results of our calculations remain almost identical. On the contrary, the values for the linear coefficients $e_{14}$ reported in Ref. 14 are close to those reported in Refs. 11 and 12 whereas the quadratic coefficients $B_{114}$ and $B_{156}$ clearly deviate. According to Ref. 14 the hybrid-functional approach they use in their DFT calculations allows a more accurate evaluation of structural parameters compared the local density approximation applied in Refs. 11 and 12. This is of particular importance for the case of low band gap (zinc-blende) III-V compounds as the latter can predict a negative band gap

| | compound | $e_{14}$ (C/m$^2$) | $B_{114}$ (C/m$^2$) | $B_{124}$ (C/m$^2$) | $B_{156}$ (C/m$^2$) |
|---|---|---|---|---|---|
| G. Bester *et al* [11] | GaAs | -0.23 | -0.439 | -3.765 | -0.492 |
| | InAs | -0.115 | -0.531 | -4.076 | -0.12 |
| A. Beya-Wakata *et al* [12] | GaAs | -0.238 | -0.4 | -3.8 | -0.7 |
| | InAs | -0.115 | -0.6 | -4.1 | 0.2 |
| G. Tse *et al* [13] | GaAs | -0.16 | -0.666 | -1.646 | neglected |
| | InAs | -0.045 | -0.653 | -1.617 | neglected |
| M. A. Caro *et al* [14] | GaAs | -0.205 | -0.99 | -3.21 | -1.28 |
| | InAs | -0.111 | -1.17 | -4.31 | -0.46 |

TABLE II: Values for the linear and quadratic piezoelectric coefficients $e_{14}$, $B_{114}$, $B_{124}$ and $B_{156}$ reported by G. Bester *et al* [11], A. Beya-Wakata *et al* [12] (only values obtained via local density approximation DFT), G. Tse *et al* [13] and M. A. Caro *et al* [14] for InAs and GaAs.

for these materials, preventing the calculation of a meaningful electric polarization (and therefore correct evaluation of the PECs). The implementation of the PECs calculated by Ref. 14 lead to an even better agreement with the experiment in terms of the stress-induced shift of the $X$ built-in dipole moment but produces a significantly different magnitude at $S_1 + S_2 = 0$ (compared to Refs. 11, 12 and 13). For this reason, we have shown in the main text the calculation obtained with the parameters of Ref. 11 which still lead to the best agreement in terms of magnitude and slope of the change of the dipole with the applied stress.
However, our results are clearly robust against the different piezoelectric coefficients reported in the literature and demonstrate unequivocally that the experimentally observed stress-dependency of the exciton built-in dipole moment cannot be reproduced without considering non-linear piezoelectric effect.

## VII. EFFECT OF SELF-CONSISTENCY CALCULATIONS

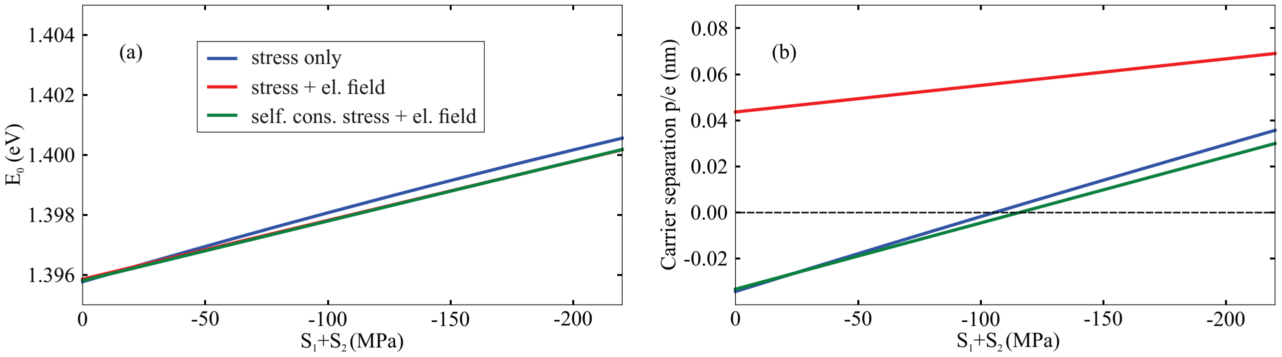


FIG. 8: (a) Emission energy and (b) carrier separation $p/e$ in studied QDs. The dependencies for the calculation when applied stress, the associated electric field $F_{qd}$ (red line), and that incorporating also the self-consistent correction (green line) are shown. In addition we show for comparison the calculation when only the applied external stress was present (blue line). All calculations were performed for $\alpha = 55°$. Note that the data for applied stress without inclusion of electric field and that when the self-consistency correction was included are very similar.


[1] R. Trotta, P. Atkinson, J. D. Plumhof, E. Zallo, R. O. Rezaev, S. Kumar, S. Baunack, J. R. Schröter, A. Rastelli, and O. G. Schmidt, Adv. Mater. **24**, 2668 (2012), URL `http://dx.doi.org/10.1002/adma.201200537`.
[2] R. Trotta, E. Zallo, E. Magerl, O. G. Schmidt, and A. Rastelli, Phys. Rev. B **88**, 155312 (2013), URL `http://link.aps.org/doi/10.1103/PhysRevB.88.155312`.
[3] R. Trotta, J. Martín-Sánchez, I. Daruka, C. Ortix, and A. Rastelli, Phys. Rev. Lett. **114**, 150502 (2015), URL `http://link.aps.org/doi/10.1103/PhysRevLett.114.150502`.
[4] R. Trotta, J. Martín-Sánchez, J. S. Wildmann, G. Piredda, M. Reindl, C. Schimpf, E. Zallo, S. Stroj, J. Edlinger, and A. Rastelli, Nat. Commun. **7**, 10375 (2016), URL `http://dx.doi.org/10.1038/ncomms10375`.

[5] M. Gong, B. Hofer, E. Zallo, R. Trotta, J.-W. Luo, O. G. Schmidt, and C. Zhang, Phys. Rev. B **89**, 205312 (2014), URL http://link.aps.org/doi/10.1103/PhysRevB.89.205312.
[6] K. K. Ng, *Complete guide to semiconductor devices* (McGraw-Hill, New York, 1995).
[7] A. M. Cowley and S. M. Sze, J. Appl. Phys. **36**, 3212 (1965), URL http://scitation.aip.org/content/aip/journal/jap/36/10/10.1063/1.1702952.
[8] Y. Zhang, Y. Liu, and Z. L. Wang, Adv. Mater. **23**, 3004 (2011), URL http://dx.doi.org/10.1002/adma.201100906.
[9] S. A. Loureno, I. F. L. Dias, J. L. Duarte, E. Laureto, L. C. Poças, D. O. Toginho Filho, and J. R. Leite, Braz. J. Phys. **34**, 517 (2004), URL http://www.scielo.br/scielo.php?script=sci_arttext&pid=S0103-97332004000300031&nrm=iso.
[10] S. Kumar, E. Zallo, Y. H. Liao, P. Y. Lin, R. Trotta, P. Atkinson, J. D. Plumhof, F. Ding, B. D. Gerardot, S. J. Cheng, et al., Phys. Rev. B **89**, 115309 (2014), URL http://link.aps.org/doi/10.1103/PhysRevB.89.115309.
[11] G. Bester, X. Wu, D. Vanderbilt, and A. Zunger, Phys. Rev. Lett. **96**, 187602 (2006), URL http://link.aps.org/doi/10.1103/PhysRevLett.96.187602.
[12] A. Beya-Wakata, P.-Y. Prodhomme, and G. Bester, Phys. Rev. B **84**, 195207 (2011), URL https://link.aps.org/doi/10.1103/PhysRevB.84.195207.
[13] G. Tse, J. Pal, U. Monteverde, R. Garg, V. Haxha, M. Migliorato, and S. Tomić, J. Appl. Phys. **114**, 073515 (2013), URL http://dx.doi.org/10.1063/1.4818798.
[14] M. A. Caro, S. Schulz, and E. P. O'Reilly, Phys. Rev. B **91**, 075203 (2015), URL http://link.aps.org/doi/10.1103/PhysRevB.91.075203.
